# Supplementary material for: Predicting commuter flows in spatial networks using a radiation model based on temporal ranges
Source: arXiv:1410.4849 ancillary file (2014-10-17)
Supplement: Supplementary file 1 [file Supplementary_Information.compressed.pdf]

## Supplementary Figures

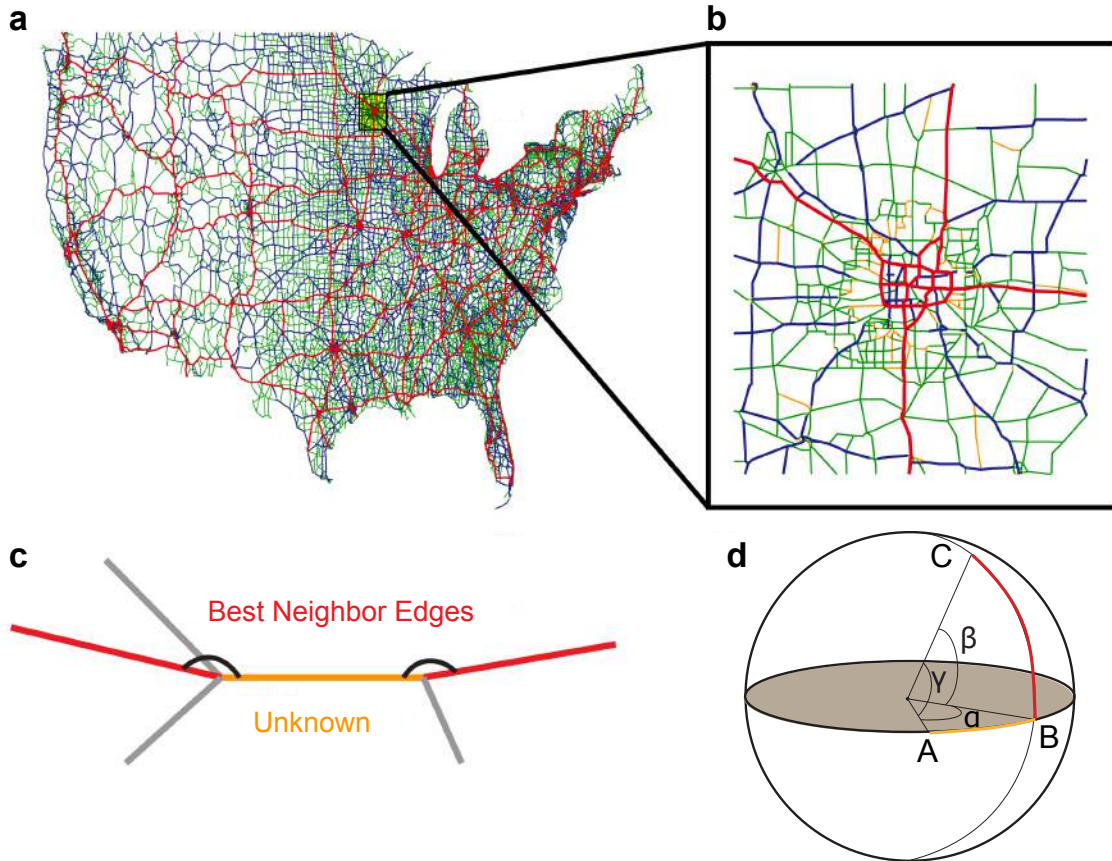

Supplementary Figure 1: Assigning ranks to edges. **(a)** Coloring edges by their road ranks. Red lines (road-rank-1) are interstate highways having road classes 1 and 11, respectively. Blue lines (road-rank-2) are inner-state freeways with road classes 2 and 12. Green lines are all the other roads. Roads with unknown road-rank are colored orange (see ref 1 for comparison). **(b)** Zooming into Minneapolis area. **(c)** Schematic for how to choose the best neighbor edges in 2D. **(d)** A schematic for calculating the alignment factor  $r$  from central angles.

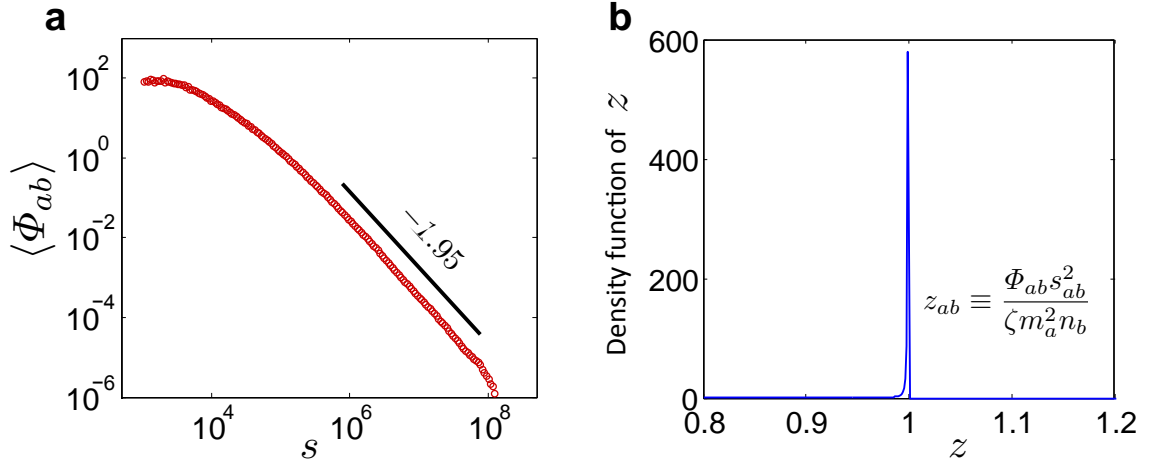

Supplementary Figure 2: **(a)** The scaling  $\Phi \sim s^{-2}$  shown as the average flux between all source destination pairs with  $s_{ab} \in [s, s + ds)$  as function of  $s$ . Alternatively, **(b)** shows the density function of  $z = \Phi_{ab} s_{ab}^2 / (\zeta m_a^2 n_b)$  which is sharply concentrated near unity. The calculations were done using time-based costs without capacity limitation and a range limit of 100 mins.

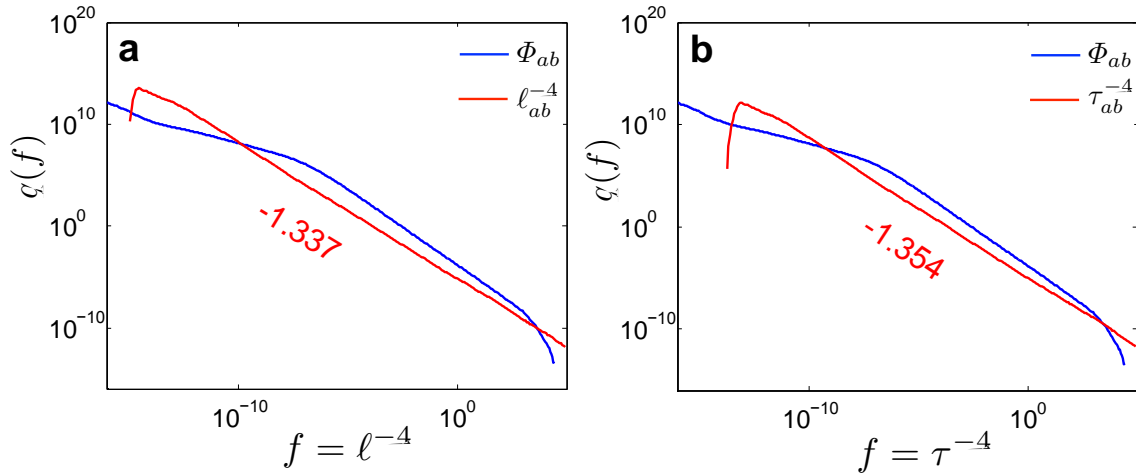

Supplementary Figure 3: The distributions  $\varrho(f)$  of  $f_{ab} = c_{ab}^{-4}$  on the roadway network. **(a)** For distance based costs  $c_{ab} = \ell_{ab}$  and **(b)** For time based costs  $c_{ab} = \tau_{ab}$ .

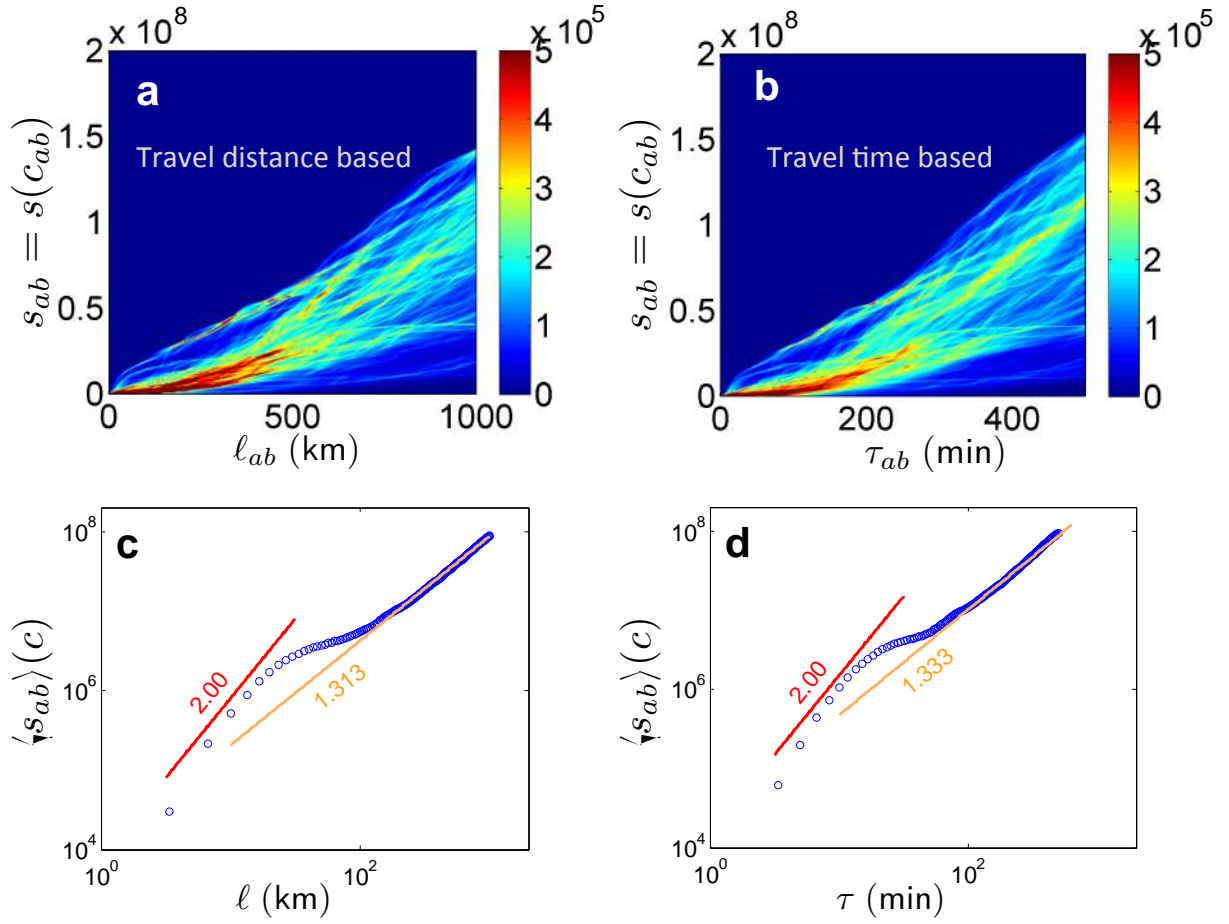

Supplementary Figure 4: The scaling of the population size  $s_{ab}$  with  $c_{ab}$ . (a) and (b) are travel distance and travel time based heat-maps. (c) and (d) are the corresponding averages, by cost.

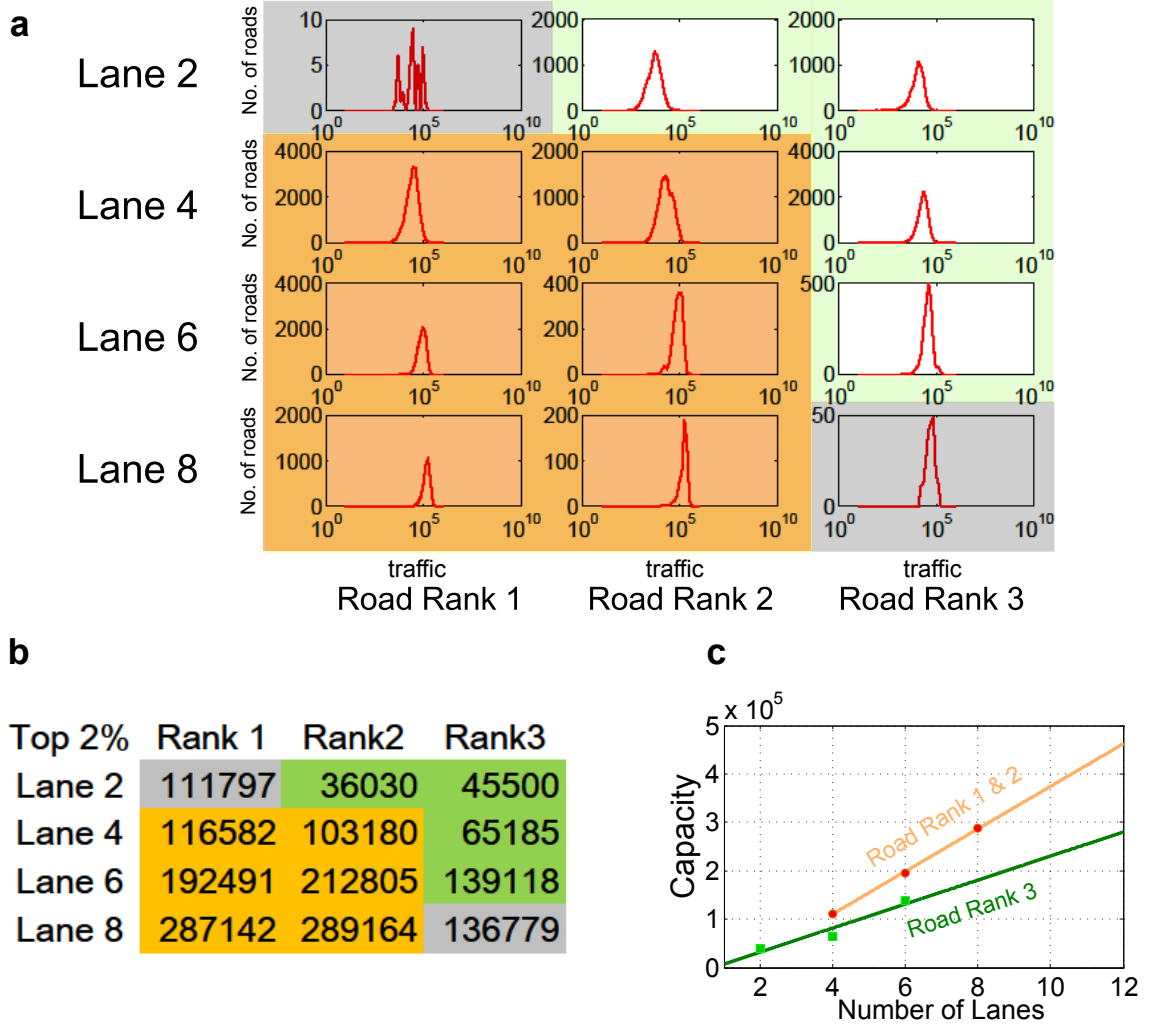

Supplementary Figure 5: Assigning edge capacities. **(a)** Distributions of real traffic (absolute values in vehicles/day averaged over 365 days) by road rank and number of lanes. The 2-lane-rank-1 and 8-lane-rank-3 cases are eliminated (masked in grey) because of sparse data. The other categories are grouped into two sets, fast group (masked in orange) and slow group (masked in green) by comparing their distributions. We assume a certain amount ( $x\%=2\%$ ) of roads in each category congested, which show up in the large traffic tail of each distribution. **(b)** By averaging the top 2% traffic from each category, we obtained an estimated road capacity for that category. **(c)** We can use these values to estimate by simple extrapolation the road capacities for other road rank-and-lane combinations not shown in **(a)**.

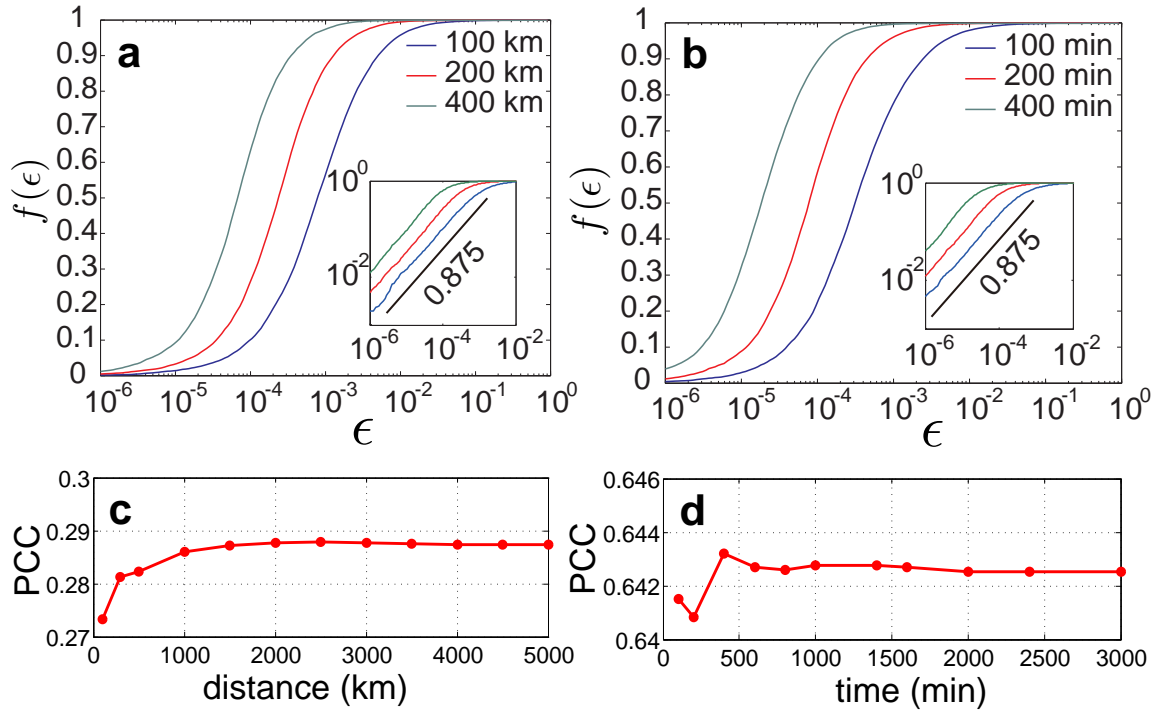

Supplementary Figure 6: **(a,b)** Cumulative fraction  $f(\epsilon)$  of nodes with relative fraction of long-range travelers not larger than  $\epsilon$ , when computing fluxes with range limitation using travel distances **(a)** and travel time **(b)**. Insets: same as the main curves, but in log-log scale showing a power-law behavior before saturation. **(c,d)** PCC computed between model and data traffic as function of range limit for travel distance **(c)** and travel time **(d)**.

## Supplementary Tables

| Speed (mph) | PCC 100min | PCC 400min |
|-------------|------------|------------|
| 75-40-15    | 0.6297     | 0.6357     |
| 75-40-20    | 0.6146     | 0.6227     |
| 75-40-10    | 0.6450     | 0.6482     |
| 75-45-15    | 0.6266     | 0.6337     |
| 75-45-20    | 0.6118     | 0.6211     |
| 75-45-10    | 0.6414     | 0.6457     |
| 75-35-15    | 0.6316     | 0.6362     |
| 75-35-20    | 0.6156     | 0.6223     |
| 75-35-10    | 0.6473     | 0.6491     |

Supplementary Table I: Speed combinations and their PCCs. We fix the rank-1 travel speed to 75 mph. First we take the travel speed combination 75-40-15 (mph), and then tune the other two speeds of road-rank-2 and 3, by  $\pm 5$  mph each. When increasing the range limit from 100 mins to 400 mins, the PCCs increase slightly and the gaps between different settings slightly shrink.

| LANES<br>CLASS | 2      | 4      | 6      | 8      |
|----------------|--------|--------|--------|--------|
| 1              | 0.0010 | 0.8942 | 0.0771 | 0.0145 |
| 2              | 0.5436 | 0.4319 | 0.0073 | 0.0004 |
| 6              | 0.6639 | 0.3069 | 0.0083 | 0.0000 |
| 7              | 0.7798 | 0.2202 | 0.0000 | 0.0000 |
| 8              | 1.0000 | 0.0000 | 0.0000 | 0.0000 |
| 9              | 1.0000 | 0.0000 | 0.0000 | 0.0000 |
| 11             | 0.0013 | 0.3890 | 0.3526 | 0.1491 |
| 12             | 0.0416 | 0.5869 | 0.2266 | 0.0721 |
| 14             | 0.2625 | 0.5537 | 0.1137 | 0.0127 |
| 16             | 0.4169 | 0.4744 | 0.0460 | 0.0000 |
| 17             | 0.6202 | 0.2837 | 0.0192 | 0.0000 |
| 19             | 0.8099 | 0.1479 | 0.0141 | 0.0000 |

Supplementary Table II: Probabilistic relations between edge classes and road lanes obtained from data. Probabilities have been normalized for each road class (summation of each row gives unity). Columns (road lanes) with very low probability were removed, in particular those with lanes-1,3,5,7, and 9–15.

## Supplementary Note 1: A brief derivation of the radiation model

The radiation model is a simple socio-demographic model of demand-supply dynamics that generates travel fluxes between all source-destination pairs. To compute the average number of commuters between a source  $a$  and destination  $b$ , the model uses extremal probability arguments, briefly described below (for details and validation see ref 2). An agent from a source  $a$  with population  $m_a$  is searching for the closest site that meets her expectations. The level of expectation or need is modeled with a scalar variable  $z$  and it is associated with the agent. It can represent an aggregate value of a wanted job position such as salary, benefits, the value or price of a delivery product, etc. Every site is associated with a value  $z'$  which represents the value of the local offer. For example, the aggregate value in terms of salary and benefits of a job offered at that site, the price the site is willing to offer for a product, etc. The agent will travel to the closest site that has an offer value that is at least as large as her expectation,  $z' \geq z$ . The original radiation model uses the simple Euclidean distance to determine closeness, but as described in the main text, a better model is one where closeness is determined by a general travel cost function, which depends on the travel modality, including the paths available for travel. The later couples the network of paths with the flux generation law. Thus, in the following we will assume that  $s_{ab}$  denotes the size of the population that can be reached within the cost of travel  $c_{ab}$  between the source  $a$  of population  $m_a$  and destination  $b$  of population  $n_b$ . It is assumed that both  $z$  and  $z'$  are drawn from the same probability distribution  $p(z)$ . Let us denote by  $q(z)$  the probability that an offer does not get accepted by our agent who has a value  $z$ . We have:  $q(z) = \int_0^z dz' p(z')$  which is just the probability that the offerer comes up with a  $z' < z$ . Due to normalization  $q(\infty) = 1$ . Then the probability that our agent with a  $z$  value will only find an acceptable offer at site  $b$  and *not at* her home-site  $a$  nor anywhere within  $s_{ab}$  is given by the product of probabilities:  $P_{m_a-1}(z)P_{s_{ab}}(z)[1 - P_{n_a}(z)]$ , where  $P_k(z)$  denotes the probability that from a population of  $k$  members none of them is making an offer acceptable to our agent:

$$P_k(z) = [q(z)]^k. \quad (1)$$

Since the agent with  $z$  is not special in any way, we need to compute the probability that any agent from  $a$  will generate such a  $z$ . This happens with probability:  $\binom{m_a}{1}p(z) = m_a p(z)$ . Collecting all, the probability that an agent will have to travel from  $a$  to destination  $b$  to meet her expectations is given by:

$$\begin{aligned} P(1|m_a, n_b, s_{ab}) &= m_a \int_0^\infty dz p(z) P_{m_a-1}(z) P_{s_{ab}}(z) [1 - P_{n_a}(z)] \\ &= m_a \int_0^\infty dz p(z) [q(z)]^{m_a+s_{ab}-1} \{1 - [q(z)]^{n_b}\} \end{aligned}$$

From the expression for  $q(z)$  it follows that  $dz p(z) = dq$  and the integral above becomes:

$$\begin{aligned} P(1|m_a, n_b, s_{ab}) &= m_a \int_0^1 dq q^{m_a+s_{ab}-1} (1 - q^{n_b}) = \int_0^1 dq q^{m_a+s_{ab}-1} - \int_0^1 dq q^{m_a+s_{ab}+n_b-1} \\ &= \frac{1}{m_a + s_{ab}} - \frac{1}{m_a + n_b + s_{ab}} = \frac{m_a n_b}{(m_a + s_{ab})(m_a + n_b + s_{ab})}. \end{aligned} \quad (2)$$

Then, the average number of individuals traveling from  $a$  to  $b$  will then be:  $\Phi_{ab} = \zeta m_a P(1|m_a, n_b, s_{ab})$ . Note that this result is independent on the form of  $p(z)$ . The exponent of 2 in the  $s_{ab}^{-2}$  scaling behavior for large  $s_{ab}$  ( $s_{ab} \gg m_a, s_{ab} \gg n_b$ ) is the result of having two integration terms in (2).

## Supplementary Note 2: Scaling properties of the mobility flux

As shown in the main text, the distribution of the traffic fluxes in the contiguous US obeys a power law  $n(\Phi) \sim \Phi^{-\mu}$  with  $\mu \simeq 1.48$  for nine orders of magnitude. Based on the extended radiation law given by Eq (1) of the main text, we expect that this scaling behavior is the consequence of the *geometrical* distribution of the population, and in particular of the growth of the population  $s_{ab}$  within the ameboid domain determined by the cost of travel  $c_{ab}$  when traveling from  $a$  to  $b$ . As discussed in the main text from the point of view of the scaling behavior, one can assume that  $s_{ab}$  is much larger than the population at any of the sites  $a$  or  $b$ , and that we can also replace the size of the population at any node (roadway intersection) with its average  $\langle m \rangle$ , see Supplementary Figure 2. Thus we only need to study the scaling behavior of

$$\Phi_{ab} \simeq \zeta m_a^2 n_b s_{ab}^{-2} \simeq \zeta \langle m \rangle^3 s_{ab}^{-2} , \quad (3)$$

There are two possible approaches we can take to compute the scaling of (3). The simplest one, which in this case is also the correct one, is to express  $s_{ab}$  as function of the number of nodes  $k$  in the Minimum Paths Tree (MPT) between  $a$  and  $b$ :  $s_{ab} \simeq \langle m \rangle k$ ,  $\rightarrow \Phi_{ab} \simeq \zeta \langle m \rangle k^{-2} \sim k^{-2}$  and proceed as described in the main text, using the fact that the distribution of the node index  $k$  (ordering statistics) is uniform. A more complicated, second approach would be to assume that

$$s_{ab} \sim \sigma \varrho c_{ab}^2 \quad (4)$$

where  $\sigma$  is the average population density and  $\varrho$  a numerical factor,  $\varrho = \mathcal{O}(1)$ . This is based on the assumption that  $s_{ab}$  is a surface area whose linear size is proportional to  $c_{ab}$ . For example, in the original radiation law we would have  $c_{ab} = r_{ab}$  and  $\varrho = \pi$ , assuming that the area covered by  $a$  and  $b$  are negligible compared to  $s_{ab}$ . Thus, one needs to study the scaling of:

$$\Phi_{ab} \simeq \frac{\zeta \langle m \rangle^3}{\varrho^2 \sigma^2} c_{ab}^{-4} \sim c_{ab}^{-4} . \quad (5)$$

However, when plotting the scaling of  $c_{ab}^{-4}$  for distance-based costs  $c_{ab} = \ell_{ab}$  and time-based costs  $c_{ab} = \tau_{ab}$  on the real roadway network, we find that both are power-laws with an exponent of about  $-1.33$  and  $-1.35$ , respectively, see Supplementary Figure 3, and not with an exponent of  $1.5$ .

Where the differences between the exponents originates from? The assumption in the second method we made was that the population  $s_{ab}$  covered within a cost  $c_{ab}$  scales as  $s_{ab} \sim c_{ab}^2$ . This is equivalent to assuming that the population  $s_{ab}$  occupies a domain with relatively smooth boundaries that can well be approximated by a square/circular patch of linear size  $c_{ab}$ . However, we show next that this is not the case. The heat-maps in Supplementary Figures 4a,b plot the growth of  $s_{ab}$  as function of  $c_{ab}$  for fixed  $a$  and all  $b$ , and for all sources  $a$ . Panel a) is for  $c_{ab} = \ell_{ab}$  and b) is for  $c_{ab} = \tau_{ab}$ . We then computed the population average  $\langle s \rangle$  within bins  $[c, c + dc]$  and plotted those in Supplementary Figures 4c,d as function of the cost  $c$ . It shows that as the cost increases, the scaling deviates significantly from  $s_{ab} \sim c_{ab}^2$  (which almost holds at low costs) to one that is approximately  $s_{ab} \sim c_{ab}^{1.3}$ , in both cases. This anomalous exponent comes from the fact that with increasing costs, the population  $s_{ab}$  occupies fractal-like domains with increasing jaggedness along its border (see also Figures 2c,d in the main paper).

## Supplementary Method 1: Computing the travel cost measure $c_{ab}$

### Travel distance based cost $\ell_{ab}$

Travel costs based on physical distance  $c_{ab} = \ell_{ab}$  are the sum of the lengths of the road segments (in km-s) along the path for which this sum is minimum between the source  $a$  and destination  $b$ . The lengths of the segments (edges) are part of the dataset and we used Dijkstra's algorithm with priority queue<sup>4</sup> to find the path with the smallest total length on the network from source to destination.

### Travel time based cost $\tau_{ab}$

In order to compute travel times, we need to estimate average traveling speeds on all the road segments. Note that speed limits do not reflect actual average traveling speeds, as they are influenced by various factors, such as traffic status, traffic lights, accidents, partial road closures, etc. But how do we estimate average traveling speeds? As we do not have direct access to such data, we use a simple approach, in which we group traveling speeds into three categories, only: fast, medium and slow. This simplistic categorization is also prompted by our desire to avoid using too many fitting parameters in our modeling. Our database contains so-called "functional classes"\*, associating a class identifier from 1 to 12 to almost all road segments in the database. These classes do not identify actual traveling speeds but allow a relative comparison between roads with fast, medium and slow travel speeds, as described below.

In the following we will use the wording "road rank" to refer to travel speed categories. Based on the info included in the functional class descriptions one can make the following categorization. The group road-rank-1 with highest speeds is formed by the interstate highways corresponding to road-class-1 and road-class-11. The medium group road-rank-2 is formed by freeways corresponding to road-class-2 and road-class-12. The rest of roads are assigned road-rank-3, see Supplementary Figure 1a. After all roads have been assigned a road rank value and an associated average traveling speed, we can use these speeds and the length of the roads to obtain average traveling times along the road segments. Then, just like in the case of travel distance based costs we identify the path in the network from source to destination that has the smallest total sum  $\tau_{ab}$  of the traveling times along its segments (edges).

Our database is incomplete and we do not know the road-class (and consequently the road-rank) for approximately 12.1% of road segments. Therefore, an important task is to predict the road ranks of these segments, a procedure which is described next.

### Estimating Edge Ranks

The idea is based on a simple machine learning approach: we identify from the part of the dataset that has complete information (87.9%) a strong predictor variable for road-rank, which is then applied on the segments with missing road-rank information. The goodness of the predictor variable is tested on the existing dataset, where we remove a fraction of the road-class data, then we apply the prediction on the segments with the artificially removed information and check to see how well we were able to reproduce the actual values.

After careful examination of the road maps (see for example the area around Minneapolis in Supplementary Figure 1b), we can make two observations. First, if two adjacent edges are lining-up, they are more likely to have the same rank. Second, if two lined-up adjacent edges have a road-rank difference,

---

\*The Functional Class represents the assigned classification from the 1992 Functional Reclassification by State agencies. Note: FHWA no longer supports the updating of FCLASS. Source: FHWA

then the difference should be at most unity (gradual change). These observations form the basis of our method. For simplicity of the argument let us assume momentarily that our geographic network is embedded in a 2D plane. (In reality it is embedded on the surface of the Earth, an oblate spheroid.) Given an edge with unknown road-rank, with multiple adjacent edges on both sides, we first determine which two of the neighbor edges ("left-best-neighbor" and "right-best-neighbor") are most lined up with the target edge in the middle, see Supplementary Figure 1c. Then, we only use these two selected edges to perform the estimation:

1. If left-best-neighbor and right-best-neighbor have the same rank, assign this rank.
2. If one of the two best neighbor edges of the target edge has unknown road-rank, we assign the road rank of the other best neighbor edge to it.
3. If rank difference is 2, namely, one has rank-3 and the other rank-1, assign rank-2.
4. If rank difference is 1:
  - (a) If road-rank-3 and road-rank-2, assign 50% road-rank-3 and 50% road-rank-2, randomly.
  - (b) If road-rank-2 and road-rank-1, assign 24% road-rank-1 and 76% road-rank-2, randomly.

In the last case, the percentages come from the ratio of corresponding road ranks in the training set. After testing on the known dataset, we obtained a correctness rate of 90.0%, which is the fraction of the correctly estimated edges from the known data. We then apply this method on the 12.1% of edges with missing road-rank information.

However, since the coordinates of edges are latitudes and longitudes, which describe positioning on a spheroid surface, it takes a little more effort to determine the best neighbor edges. We define  $r$  as the alignment factor of two adjacent line segments:  $r = \gamma / (\alpha + \beta)$  where  $\alpha$  and  $\beta$  are the central angles of the two adjacent edges (arcs AB and BC in Supplementary Figure 1d) and  $\gamma$  is the central angle between the non-connected end points (between A and C in Supplementary Figure 1d). If the two segments (AB and BC) would be lining up perfectly, we would have  $\alpha + \beta = \gamma$  and  $r$  would reach the maximum value of 1. Given the geographical coordinates (lat and long) of two points  $(\phi_1, \theta_1)$  and  $(\phi_2, \theta_2)$  the central angle  $\alpha$  between them can be calculated via:

$$\alpha = \arccos(\sin \phi_1 \sin \phi_2 + \cos \phi_1 \cos \phi_2 \cos(\theta_1 - \theta_2)) \quad (6)$$

Then using (6) we can calculate all three angles  $\alpha$ ,  $\beta$  and  $\gamma$  and obtain the factor  $r$  between the target edge and all its neighbors. The neighbor with largest  $r$  will be selected on both sides and we return to the method described above.

### Assigning Travel Speeds to Edge Ranks

After all road ranks have been obtained, we associate a travel speed to each road rank. The goodness of our prediction is tested using Pearson's correlation coefficient (PCC)<sup>5</sup> which tests for the linear alignment between the two datasets. Observe that the traveling speeds are scaling factors, converting edge weights from distance to time. Although there are three different traveling speeds, we only have two degrees of freedom of tuning, because the PCC is invariant against overall changes in the scale of the variables. For example, the setting of travel speeds 9mph, 5mph and 1mph for road-rank-1, 2 and 3, respectively, will generate the same PCC as setting 90mph, 50mph and 10pmh. Therefore, we may fix one travel speed, 75 miles per hour for road rank 1, and then tune the other two.

Table I summarizes the effects of changing the average traveling speed for road ranks 2 and 3 on the PCC when using  $\tau_{ab}$  for travel costs (see also main text). The PCC varies from 0.61 to 0.64, all of which are larger than the PCC-s obtained using travel distance based costs  $\ell_{ab}$ .

## Supplementary Method 2: Estimating edge capacities

Road capacity, here defined as the maximum traffic a road segment can let through per day before congestion occurs, mainly depends on the travel speed and the number of lanes. The reader may think of this as sort of a fluid flow capacity, which depends on flow velocity and cross-section area. Our approach to estimate road capacities was to extract them from our dataset, which provides traffic values for 43% of all road segments. First, we created 12 categories formed by the combinations of the three road ranks (speeds: slow, medium and fast) and the four types of the most represented lane numbers (in the data), which are lane numbers 2, 4, 6 and 8. Note that there are other lane numbers (from 1 to 19) as well, however, they occur very rarely. We next plotted the distribution of the real traffic within each of these 12 categories, as shown in Supplementary Figure 5a.

We used the values in the tails of the traffic distributions from Supplementary Figure 5a to obtain capacity estimates. While not all roads within the same category are regularly used at maximum capacity those that are, appear in the large traffic tail of these distributions. We computed the average of the top  $x\% = 2\%$  percent of traffic values to estimate the capacity of the corresponding category (Supplementary Figure 5b). The value of  $x\%$  was chosen self-consistently to obtain the largest PCC and the best fit of the traffic distributions after iterating our flow redistribution program described in the main text.

As there are many speed and lane number combinations left out from the 12 categories in Supplementary Figure 5a, we need a way to extrapolate or interpolate to the values not in the table. As expected, as the number of lanes grow, the capacities should grow proportionately. Accordingly, we identified several groups in the table of Supplementary Figure 5a within which a linear relationship exists. This is plotted in Supplementary Figure 5c: the capacities of road ranks 1 and 2 could be polled together into a single group indicated by orange highlight in Supplementary Figure 5a-c and slow rank 3 with the corresponding lanes forming their own group, highlighted in green. The regions highlighted in grey had too sparse datasets, they were not used for extrapolation. For road segments falling into any of these twelve categories, we assigned the average of the top 2% traffic values as their capacities; for other road segments, we calculated the capacities from the fitted linear functions depending on their rank.

In our dataset 43% of the edges have information on the number of lanes (for the same set of roads for which the traffic measurements exist). However, we need to compute capacities for all roads. However, roads without traffic data did not have lane information. To estimate the number of lanes for the other edges, we applied a simple probabilistic classification method. A strong correlation between the road class feature and the number of lanes has been found, with an information gain ratio of 0.438. Information gain ratio was calculated with the help of the data mining software WEKA. Information gain is also known as Kullback-Leibler divergence, which measures the dependency of two distributions. The value goes from zero to one, larger value indicating higher dependency. Supplementary Table II shows the conditional probabilities for the occurrence of the most represented road-lane values (2, 4, 6 and 8) within every road-class, based on the part of the dataset that has this information. Since the subset of the data with lane information is fairly large and well distributed across the whole US, we may assume that these conditional probabilities are representatives of the whole dataset and they would not change significantly if lane information would be available for all the roads. Thus for every road with a given road-class we

may assign a lane number according to the conditional probabilities shown in Supplementary Table II.

## Supplementary References

1. [http://www.fhwa.dot.gov/planning/national\\_highway\\_system/](http://www.fhwa.dot.gov/planning/national_highway_system/)
2. Simini, F., Gonzalez, M.C., Maritan, A. & Barabási, A. L. *Nature* **484** 96-100 (2012).
3. <http://federalgovernmentzipcodes.us>
4. Fredman, M. L. & Tarjan, R. E. *25th Annual Symposium on Foundations of Computer Science (IEEE)*, 338-346 (1984).
5. Rodgers, J. L. & Nicewander, W. A. *The American Statistician*, **42**(1), 59 (1988).
